# Supplementary material for: Connectivity-Driven Parcellation Methods for the Human Cerebral Cortex
Source: arXiv:1802.06772 source file (2018-02-17)
Supplement: Supplementary file 1 [file appendixB.tex]

\chapter{Graph Theoretical Measures}
Graph theory has played an integral role in recent efforts to understand the structure and function of complex systems like the human brain, and has been widely used to characterize patterns and explore topological properties of connectivity networks.~\cite{watts1998collective}, particularly, focused on two key properties of a network, i.e. the clustering coefficient and the characteristic path length. The clustering coefficient is one of the most elementary measures of local segregation, which measures the density of connections between a node’s neighbours. The average of the clustering coefficients for each individual node is the clustering coefficient of the graph. Clustering is significant in a neurobiological context because neuronal units or brain regions that form a densely connected cluster or module communicate a lot of shared information and are therefore likely to constitute a functionally coherent brain system. The clustering coefficient of a binary network can be computed by:

\begin{equation}
C_i=\frac{1}{k_i(k_i-1)}\sum_{j,k \in N}(a_{ij}a_{jk}a_{ki})
\end{equation}

where \textit{N} is the set of all nodes in the network, $k_i$ is the degree of node \textit{i}, and $a_{ij}$ is connection status between \textit{i} and \textit{j}, with $a_{ij}=1$ if there is a link and $a_{ij}=0$ otherwise. The degree of a node is the number of edges attached to it and connecting  it to the rest of the network.

While clustering evaluates local connectivity and the segregation of the network into communities, another set of measures captures the capacity of the network to engage in more global interactions that transcend the boundaries of modules and enable network-wide integration. One of the most commonly used measures of integration in brain networks is the characteristic path length, usually computed as the global average of the graph’s distance matrix~\cite{watts1998collective}. The characteristic path length is a measure of functional integration of the network, demonstrating its ability to quickly combine specialised information from distributed brain regions. A short path length indicates that, on average, each node can be reached from any other node along a path composed of only a few edges. The path length between nodes $i$ and $j$ is given by:
  
\begin{equation}\label{eq:path_length}
d_{ij}=\sum_{a_{uv}\in g_{i \leftrightarrow j}}a_{uv}
\end{equation}
\kern 1em

\noindent where $g_{u \leftrightarrow v}$ is the shortest path between $u$ and $v$. However, the absolute value of the path length varies greatly with the size and density of individual graphs and, hence, provides only limited information on integration in the network. The network path length should therefore be compared to path lengths of appropriately constructed random networks. For this reason it is customary to compare the obtained path length to that of randomized reference networks with the same number of nodes and edges and identical node degrees as the original network. Such reference networks can be provided by randomizing the original network using a random switching procedure~\cite{rubinov2010complex}. The calculated values for the clustering coefficient and the path length can, then, be normalized by dividing them with the average corresponding values of the randomized networks. In this study we normalise these metrics using a set of 1000 random networks with the same degree distribution as the original ones.

An important shared feature of complex networks like the human brain is small-world topology~\cite{bullmore2009complex}. In a small-world network, most links are among neighbouring nodes, but there are a few connections to distant nodes that create shortcuts across the network. As a result, small-world networks are characterised by the prevalence of exquisitely small path lengths among pairs of nodes within very large networks.A prior belief about the small-worldness of the brain arises from the fact that it supports both segregated and distributed information and is also likely evolved to maximise efficiency and minimise the cost of information processing~\cite{bassett2006small}. The small-world index can be calculated as:

\begin{equation}
\sigma = \frac{\gamma}{\lambda}
\end{equation}

\noindent where $\gamma$ is the normalized clustering coefficient and $\lambda$ the normalized path length.
